# Supplementary material for: Components of polarization-transfer to a bound proton in a deuteron measured by quasi-elastic electron scattering
Source: arXiv:1801.01306 source file (2018-01-18)
Supplement: Supplementary file 1 [file deepCompSuppPlb.pdf]

# Components of polarization-transfer to a bound proton in a deuteron measured by quasi-elastic scattering Supplementary material

D. Izraeli*, I. Yaron, B. S. Schlimme, *et al.*, for the A1 Collaboration

**Abstract**

We provide in this supplement the kinematics and details of the experimental set-up as well as the continuous presentation of the polarization-transfer described in the paper.

Table 1: The kinematic settings in the experiment. The angles and momenta are the central values for the two spectrometers' settings: $p_p$ and $\theta_p$ ($p_e$ and $\theta_e$) are the knocked out proton (scattered electron) momentum and scattering angles, respectively.

| Kinematic | Setting | | |
|---|---|---|---|
| | A | B | D |
| $Q^2$ [GeV$^2$/c$^2$] | 0.40 | 0.4 | 0.18 |
| $E_{\mathrm{beam}}$ [MeV] | 600 | 600 | 630 |
| $p_{\mathrm{miss}}$ [MeV/c] | $-80$ to 75 | 75 to 175 | $-220$ to $-130$ |
| $p_e$ [MeV/c] | 385 | 463 | 398 |
| $\theta_e$ [deg] | 82.4 | 73.8 | 49.4 |
| $p_p$ [MeV/c] | 668 | 495 | 665 |
| $\theta_p$ [deg] | $-34.7$ | $-43.3$ | $-39.1$ |
| # of events after cuts | 210 k | 170 k | 790 k |

*Corresponding author
*Email address:* davidizraeli@post.tau.ac.il (D. Izraeli)

Table 2: Data parametrization for $P_y^{^2\mathrm{H}}$ and the ratios $P_x^{^2\mathrm{H}}/P_x^{^1\mathrm{H}}$ and $P_z^{^2\mathrm{H}}/P_z^{^1\mathrm{H}}$ (defined in the paper) as a function of the knocked out proton virtuality, for $p_{\mathrm{miss}} > 0$. $\Delta P^{^2\mathrm{H}}/P^{^2\mathrm{H}}$ is the parameterization's relative uncertainty for each of the three components. This parametrization is used in Fig. 5.

| $\nu$ $\left[\mathrm{GeV}^2/c^2\right]$ | $P_x^{^2\mathrm{H}}/P_x^{^1\mathrm{H}}$ | $P_y^{^2\mathrm{H}}$ | $P_z^{^2\mathrm{H}}/P_z^{^1\mathrm{H}}$ | $\Delta P^{^2\mathrm{H}}/P^{^2\mathrm{H}}$ |
|---|---|---|---|---|
| -0.0500 | 0.829 | 0.00049 | 0.821 | 0.060 |
| -0.0475 | 0.831 | 0.00033 | 0.819 | 0.056 |
| -0.0450 | 0.835 | 0.00042 | 0.821 | 0.053 |
| -0.0425 | 0.842 | 0.00054 | 0.825 | 0.050 |
| -0.0400 | 0.851 | 0.00076 | 0.832 | 0.048 |
| -0.0375 | 0.861 | 0.00106 | 0.840 | 0.045 |
| -0.0350 | 0.871 | 0.00094 | 0.850 | 0.042 |
| -0.0325 | 0.882 | 0.00115 | 0.862 | 0.038 |
| -0.0300 | 0.895 | 0.00121 | 0.874 | 0.035 |
| -0.0275 | 0.907 | 0.00137 | 0.887 | 0.031 |
| -0.0250 | 0.919 | 0.00159 | 0.900 | 0.027 |
| -0.0225 | 0.931 | 0.00129 | 0.913 | 0.024 |
| -0.0200 | 0.941 | 0.00133 | 0.926 | 0.022 |
| -0.0175 | 0.952 | 0.00159 | 0.938 | 0.020 |
| -0.0150 | 0.964 | 0.00213 | 0.951 | 0.019 |
| -0.0125 | 0.976 | 0.00233 | 0.965 | 0.019 |
| -0.0100 | 0.985 | 0.00265 | 0.978 | 0.019 |
| -0.0075 | 0.989 | 0.00178 | 0.987 | 0.019 |
| -0.0050 | 0.989 | 0.00062 | 0.992 | 0.019 |
| -0.0025 | 0.983 | 0.00097 | 0.992 | 0.018 |
| 0.0000 | 0.973 | 0.00087 | 0.984 | 0.018 |

Table 3: Data parametrization (see caption of Tab. 2) as a function of the knocked out proton virtuality, for $p_{\text{miss}} < 0$. This parametrization is used in Fig. 5.

| $\nu$ $\left[\text{GeV}^2/c^2\right]$ | $P_x^{^2\text{H}}/P_x^{^1\text{H}}$ | $P_y^{^2\text{H}}$ | $P_z^{^2\text{H}}/P_z^{^1\text{H}}$ | $\Delta P^{^2\text{H}}/P^{^2\text{H}}$ |
|---|---|---|---|---|
| -0.1050 | 1.065 | 0.00273 | 1.787 | 0.046 |
| -0.1025 | 1.102 | 0.00408 | 1.804 | 0.043 |
| -0.1000 | 1.133 | 0.00417 | 1.809 | 0.041 |
| -0.0975 | 1.155 | 0.00401 | 1.803 | 0.039 |
| -0.0950 | 1.171 | 0.00355 | 1.788 | 0.037 |
| -0.0925 | 1.184 | 0.00333 | 1.770 | 0.035 |
| -0.0900 | 1.192 | 0.00328 | 1.744 | 0.032 |
| -0.0875 | 1.195 | 0.00391 | 1.714 | 0.030 |
| -0.0850 | 1.196 | 0.00366 | 1.683 | 0.027 |
| -0.0825 | 1.196 | 0.00340 | 1.653 | 0.026 |
| -0.0800 | 1.193 | 0.00322 | 1.619 | 0.025 |
| -0.0775 | 1.190 | 0.00355 | 1.588 | 0.025 |
| -0.0750 | 1.187 | 0.00319 | 1.559 | 0.025 |
| -0.0725 | 1.184 | 0.00358 | 1.531 | 0.025 |
| -0.0700 | 1.183 | 0.00322 | 1.508 | 0.025 |
| -0.0675 | 1.185 | 0.00349 | 1.489 | 0.024 |
| -0.0650 | 1.189 | 0.00298 | 1.474 | 0.022 |
| -0.0625 | 1.196 | 0.00280 | 1.465 | 0.021 |
| -0.0600 | 1.206 | 0.00246 | 1.460 | 0.019 |
| -0.0575 | 1.217 | 0.00282 | 1.457 | 0.020 |
| -0.0550 | 1.226 | 0.00251 | 1.452 | 0.022 |
| -0.0525 | 1.228 | 0.00257 | 1.441 | 0.023 |
| -0.0500 | 1.218 | 0.00210 | 1.415 | 0.021 |
| -0.0475 | 1.196 | 0.00235 | 1.378 | 0.019 |
| -0.0450 | 1.172 | 0.00214 | 1.339 | 0.022 |
| -0.0425 | 1.156 | 0.00168 | 1.310 | 0.024 |
| -0.0400 | 1.155 | 0.00151 | 1.299 | 0.022 |
| -0.0375 | 1.160 | 0.00119 | 1.296 | 0.020 |
| -0.0350 | 1.158 | 0.00058 | 1.284 | 0.023 |
| -0.0325 | 1.141 | 0.00047 | 1.258 | 0.026 |
| -0.0300 | 1.111 | 0.00009 | 1.218 | 0.027 |
| -0.0275 | 1.073 | 0.00026 | 1.170 | 0.027 |
| -0.0250 | 1.033 | 0.00040 | 1.121 | 0.027 |
| -0.0225 | 0.993 | 0.00093 | 1.080 | 0.028 |
| -0.0200 | 0.949 | 0.00385 | 1.047 | 0.029 |
| -0.0175 | 0.920 | 0.00600 | 1.017 | 0.030 |
| -0.0150 | 0.910 | 0.00510 | 0.992 | 0.028 |
| -0.0125 | 0.912 | 0.00398 | 0.980 | 0.026 |
| -0.0100 | 0.920 | 0.00253 | 0.974 | 0.023 |
| -0.0075 | 0.932 | 0.00181 | 0.971 | 0.020 |
| -0.0050 | 0.946 | 0.00059 | 0.968 | 0.018 |
| -0.0025 | 0.960 | 0.00078 | 0.974 | 0.017 |
